# Supplementary material for: Training and Evaluation of Deep Policies using Reinforcement Learning and Generative Models
Source: arXiv:2204.08573 source file (2022-04-18)
Supplement: Supplementary file 1 [file appendix.tex]

\begin{appendices}

\section{End-to-end Training of Perception and Control}
\label{sec:perception}
The EM policy training algorithm presented in Section~\ref{sec:em_policy_training} updates the deep policy using the supervised learning objective function introduced in~\eqref{eq:M_loss} (the M-step objective). 
Similar to GPS \cite{levine2016end}, the EM policy training formulation enables simultaneous training of the perception and control parts of the deep policy in an end-to-end fashion. 
In this section, we describe two techniques that can improve the efficiency of the end-to-end training.

\textbf{Input remapping trick}
The input remapping trick \cite{levine2016end} can be applied to condition the variational policy $q$ on a low-dimensional compact state representation, $z$, instead of the high-dimensional states $s$ given by the sensory observations, e.g., camera images. 
The policy training phase can be done in a controlled environment such that extra measures other than the sensory observation of the system can be provided. These extra measures can be for example the position of a target object on a tabletop. 
Therefore, the image observations $s$ can be paired with a compact task-specific state representation $z$ such that $z$ is used in the E-step for updating the variational policy $q_\phi(\alpha|z)$, and $s$ in the M-step for updating the policy $\pi_\theta(\alpha|s)$. 

\textbf{Domain adaptation for perception training}
%The unlabeled images, captured without involving the robot, can be used to improve the data-efficiency of the visuomotor policy training. 
Domain adaptation techniques, e.g., adversarial methods \cite{chen2019adversarial}, can improve the end-to-end training of visuomotor policies with limited robot data samples. 
The unlabeled task-specific images, captured without involving the robot, can be exploited in the M-step to improve the generality of the visuomotor policy to manipulate novel task objects in cluttered backgrounds. 

The M-step is updated to include an extra loss function to adapt data from the two different domains: (i) unlabeled images and (ii) robot visuomotor data. 
The images must contain only one task object in a cluttered background, possibly different than the task object used by the robot during the policy training. 
Given images from the two domains, the basic idea is to extract visual features such that it is not possible to detect the source of the features. 
More details of the method can be found in our recent work in \cite{chen2019adversarial}.

\section{Disentangling Precision and Recall} \label{app:dis_score}
Let $l \in \{1, \dots, N_\alpha\}$ be a fixed latent dimension. In phase $1$, we perform $D \in \mathbb{N}$ interventions $\alpha_l = I_d$ on the latent dimension $l$ where $d = 1, \dots, D$. Interventions are chosen from the set of equidistant points on the interval $[-a, a]$ such that $I_d = -a + 2a \cdot \frac{d-1}{D - 1}$. The value $a$ is chosen such that $[-a, a]$ is in the support of the prior distribution $p(\alpha)$. Since $p(\alpha)$ is a standard normal distribution in the case of VAEs and a uniform distribution on the interval $[-1, 1]$ in the case of GANs, we set $a$ to be $1.5$ and $1$ in the case of the VAEs and GANs, respectively. Each intervention $d = 1, \dots, D$ is performed on $n$ samples from the prior distribution $p(\alpha)$ and yields a set of $n$ end states  denoted by $\boldsymbol{S}_g^{l-I_d}$. For each intervention we additionally randomly sample a set $\boldsymbol{S}_r$ of $n$ end states corresponding to the training motor data. Note that elements of both $\boldsymbol{S}_g^{l-I_d}$ and $\boldsymbol{S}_r$ are $N_s$-dimensional with $N_s$ being the dimension of the end state space, which are obtained by executing the generated trajectories on the robotic platform..

In phase $2$, we calculate the $\MMD(\proj_j \boldsymbol{S}_g^{l-I_d}, \proj_j \boldsymbol{S}_r)$ for a fixed intervention $d = 1, \dots, D$ and every end state component $j = 1, \dots, N_s$. We first determine if the difference between the sets $\proj_j \boldsymbol{S}_g^{l-I_d}$ and $\proj_j \boldsymbol{S}_r$ is large enough to reject the null hypothesis that samples from $\proj_j \boldsymbol{S}_g^{l-I_d}$ and $\proj_j \boldsymbol{S}_r$ are drawn from the same distribution. We achieve this by performing a permutation test where we pool all the samples from $\proj_j \boldsymbol{S}_g^{l-I_d}$ and $\proj_j \boldsymbol{S}_r$, randomly divide the pooled set into two sets of $n$ elements and calculate the $\MMD$ between the obtained sets. The random split into two sets is performed $100$ times such that we obtain a distribution over the resulting $\MMD$ values. For a predetermined significance level $\eta$, we define the critical value $c_\eta$ to be $(1 - \eta)$-quantile of the obtained distribution over $\MMD$ values.
%significant, we first perform a permutation test to determine the critical value $c_\eta$ where $\eta$ denotes the significance level. 
We then say that the intervention $I_d$ was significant for an end state component $j$ if the observed $\MMD(\proj_j \boldsymbol{S}_g^{l-I_d}, \proj_j \boldsymbol{S}_r) > c_\eta$. The calculations in phase $2$ were repeated $p$ times with a resampled set of $n$ training end states $\boldsymbol{S}_r$. In all our experiments we set $p = 10$ and $\eta = 0.001$. 

Therefore, phases $1$ and $2$ yield functions $c_g: \{1, \dots, N_\alpha\} \longrightarrow \{1, \dots, N_s\}$ and $d_g: \{1, \dots, N_\alpha\} \longrightarrow \mathbb{R}$ defined by:
\begin{align*}
    c_g(l) = \argmax_{j = 1, \dots, N_s} \overline{\MMD}\left(\proj_j \boldsymbol{S}_g^{l-I_d}, \proj_j \boldsymbol{S}_r\right) \quad \textrm{and} \quad d_g(l) = \overline{\MMD}\left(\proj_{c_g(l)} \boldsymbol{S}_g^{l-I_d},  \proj_{c_g(l)} \boldsymbol{S}_r\right)
\end{align*}
where $\overline{\MMD}$ denotes the average $\MMD$ score calculated on a subset of $p \cdot D$ performed interventions that were significant. For a given latent dimension $l \in \{1, \dots, N_\alpha\}$, $c_g(l)$ represents the dimension of the end state space $\mathbb{R}^{N_s}$ that was most affected by the latent interventions. This is because a high $\MMD$ value indicates a low similarity between $\proj_j \boldsymbol{S}_g^{l-I_d}$ and $\proj_j \boldsymbol{S}_r$, and thus a high effect of the intervention. Moreover, $d_g(l)$ is the average $\MMD$ value obtained on the most affected end state space dimension identified by $c_g(l)$.

In phase $3$ we define the final disentanglement score for the generative model $g$ using the functions $c_g$ and $d_g$. Let $\mathcal{P}$ be a subset of $\{ d_g(l): l = 1 \dots, N_\alpha\}$ containing its largest three elements, i.e., the three largest $\overline{\MMD}$ values obtained in phase 2, and let $\mathcal{R} = \{c_g(l): d_g(l) \in \mathcal{P}\}$ be the set of the corresponding end state components. We define the \textit{Disentangling Precision and Recall} $\Dis$ as a pair
\begin{align}
    \Dis(g) = (\Dip(g), \Dir(g)) := \left(\sum_{d \in \mathcal{P}} d, \frac{|\mathcal{R}^{\neq}|}{N_s} \right)
\end{align}
where $\mathcal{R}^{\neq}$ denotes the subset of unique elements of the set $\mathcal{R}$. The \textit{disentangling recall} $\Dir$ is the fraction of end state dimensions described by three most significant latent dimensions, i.e., by the three latent dimensions on which interventions yielded the largest changes in the end state space. The larger the $\Dir$ value, the more end state space dimensions are captured in the latent space, and thus the latent disentanglement has a higher recall.
Similarly, the \textit{disentangling precision} $\Dip$ is the sum effect that the latent interventions on the three most significant latent dimensions have on the affected end state dimensions. The larger the $\Dip$, the stronger was the effect of the latent interventions, and thus the latent disentanglement is more precise.

\section{Generative models} \label{app:gen_models}
\subsection{Variational Autoencoder}
The architecture of the decoder neural network is visualised in Table \ref{tab:gen_arc}. The encoder neural network is symmetric to the decoder with two output linear layers of size $N_\alpha$ representing the mean and the log standard deviation of the approximate posterior distribution. All the models were trained for $10000$ epochs with learning rate fixed to $1e-4$.

\subsection{InfoGAN}
The architecture of the generator, discriminator and Q neural network parametrizing $Q_\phi(\alpha|\tau)$ are summarised in Tables \ref{tab:gen_arc} and \ref{tab:dis_arc}. All the models were trained for $1000$ epochs with learning rates of the optimizers for the generator and discriminator networks fixed to $2e-4$. 

\begin{table}[!htb]
    \begin{minipage}{.4\linewidth}
      \caption{Architecture of the generator neural network.} \label{tab:gen_arc}
      \centering
        \begin{tabular}{l}
         \hline
         \hline
         Linear($N_\alpha$, $128$) + BatchNorm + ReLU \\ 
         \hline
         Linear($128$, $256$) + BatchNorm + ReLU \\
         \hline
         Linear($256$, $512$) + BatchNorm + ReLU \\
         \hline
         Linear($512$, $7 \cdot 79$)
    \end{tabular}
    \end{minipage}%
    \hfill
    \begin{minipage}{.4\linewidth}
      \centering
        \caption{Architecture of the discriminator and Qnet neural networks.} \label{tab:dis_arc}
        \begin{tabular}{l|l}
         \hline
         \hline
         \multirow{2}{*}{Shared layers} & Linear($7 \cdot 79$, $256$) + ReLU \\ 
         \cline{2-2}
         & Linear($256$, $128$) + ReLU \\
         \hline
         discriminator & Linear($128$, $1$) + Sigmoid \\
         \hline \multirow{2}{*}{Qnet} & Linear($128$, $64$) \\ \cline{2-2}
          & Linear($64$, $N_\alpha$) 
         
         \end{tabular}
    \end{minipage} 
\end{table}

\end{appendices}
